# Supplementary material for: Addressing Bias in Online Selection with Limited Budget of Comparisons
Source: arXiv:2303.09205 source file (2024-11-17)
Supplement: Supplementary file 1 [file appendixExperiments.tex]

Moreover, Theorem \ref{thm:single-thresh} reveals that the asymptotic success probability is independent of the probabilities of belonging to each group, and it is equal to a value smaller than $1/e$. This indicates a discontinuity of the asymptotic success probability at the extreme points of the polygon defining the possible values of $(\lambda_k)_{k \in [K]}$. Figure \ref{fig:ST_discontinuity} illustrates this behavior for the case of two groups, with $N=500$ candidates.

\begin{figure}[h!]
    \centering
    \includegraphics[width=0.5\textwidth]{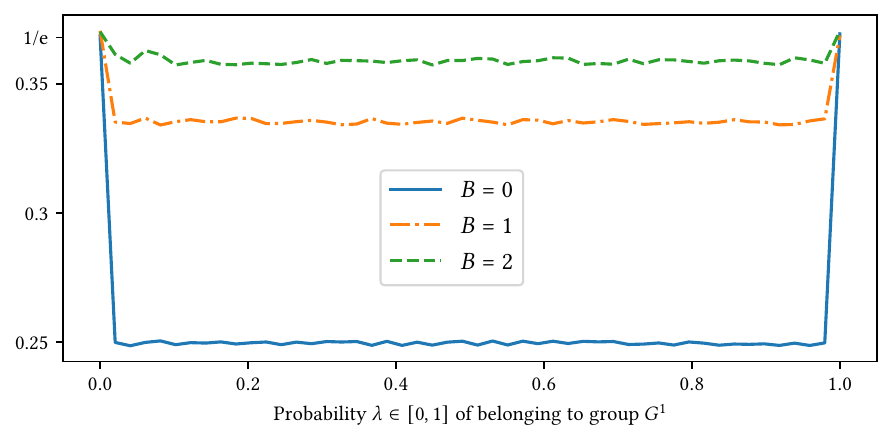} 
    \caption{Single threshold: success probability for $2$ groups, with $N = 500$ and $\lambda = \Pr(g_t = 1) \in [0,1]$}
    \label{fig:ST_discontinuity}
\end{figure}

The success probability we proved in Theorem \ref{thm:single-thresh} is only asymptotic, it is reached when the number of candidates is very high. Moreover, from Lemma \ref{lem:single-thres-recursion} and from the proof of the theorem, it can be deduced that the difference between the success probability for a given $N$ and the limit is $O\big(\sqrt{\tfrac{\log N}{N}}\big)$. However, this does not comprehend how the success probability varies with the number of candidates. Figure \ref{fig:ST_Ngrows} shows that the success probability is actually better when the number of candidates is small, and it decreases to match the asymptotic expression when $N \to \infty$, represented with dotted lines for $K \in \{2,3,4\}$.

\begin{figure}[h!]
    \centering
    \includegraphics[width=0.5\textwidth]{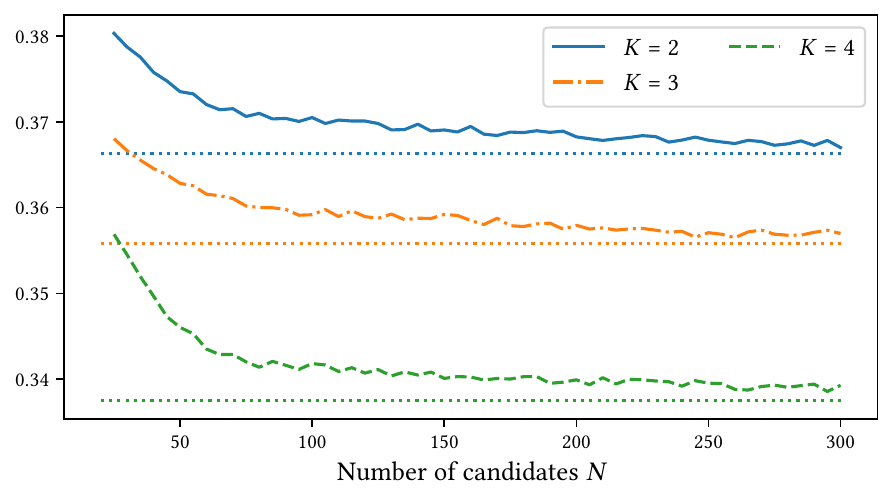} 
    \caption{Convergence to the asymptotic success probability, with $\lambda_k = 1/K$ for all $k \in [K]$}
    \label{fig:ST_Ngrows}
\end{figure}
